# Supplementary material for: A Cantor-Kantorovich Metric Between Markov Decision Processes with Application to Transfer Learning
Source: arXiv:2407.08324 source file (2024-07-11)
Supplement: Supplementary file 1 [file appendices.tex]

\section{Proof of Theorem 1} 
\section{Proof of Theorem 2}
